# Supplementary material for: Artificial life of an active droplets system: a quantitative lifecycle analysis
Source: arXiv:2511.17786 ancillary file (2025-11-21)
Supplement: Supplementary file 1 [file supp.pdf]

# Supporting information to “Artificial life of an active droplets system: a quantitative lifecycle analysis”

Matteo Scandola,<sup>1,2</sup> Silvia Holler,<sup>2</sup> Richard J. G. Löffler,<sup>3</sup> Martin M. Hanczyc,<sup>2,4,\*</sup> Raffaello Potestio,<sup>5,6,†</sup> and Roberto Menichetti<sup>5,6,‡</sup>

<sup>1</sup>*Laboratoire Jean Perrin, UMR 8237 Sorbonne Université/CNRS, Institut de Biologie Paris Seine, 4 Place Jussieu, F-75005 Paris, France*

<sup>2</sup>*Department of Cellular, Computational and Integrative Biology (CIBIO), University of Trento, via Sommarive 9, I-38123 Trento, Italy*

<sup>3</sup>*Centre for Star and Planet Formation, Globe Institute, University of Copenhagen, Copenhagen, Denmark*

<sup>4</sup>*Chemical and Biological Engineering, University of New Mexico, Albuquerque, NM, 87106, USA*

<sup>5</sup>*Physics Department, University of Trento, via Sommarive, 14 I-38123 Trento, Italy*

<sup>6</sup>*INFN-TIFPA, Trento Institute for Fundamental Physics and Applications, I-38123 Trento, Italy*

(Dated: November 21, 2025)

In this Supporting Information, we report the results of analyses analogous to those presented in the main text for all three independent experimental realizations of the system investigated in this work. More specifically, we display: (i) snapshots of the three experiments, illustrating typical droplet configurations at the onset of each evolutionary stage of the system; (ii) the temporal evolution of the velocity polarization, hexatic order parameter, and average speed of the droplets along the three experiments; (iii) the time- and species-averaged mean squared displacements of the two droplet species for the three experiments; (iv) the velocity autocorrelation functions of the two droplet species for the three experiments; (v) the turning angle distributions of the two droplet species for the three experiments; and (vi) the dimer distributions of the two droplet species for the three experiments.

## Contents

|                                                                   |          |
|-------------------------------------------------------------------|----------|
| <b>I. Experimental snapshots</b>                                  | <b>2</b> |
| <b>II. Collective variables analysis</b>                          | <b>2</b> |
| <b>III. Time- and species-averaged mean squared displacements</b> | <b>3</b> |
| <b>IV. Velocity autocorrelation functions</b>                     | <b>6</b> |
| <b>V. Turning angle distributions</b>                             | <b>7</b> |
| <b>VI. Distribution of droplets around a dimer</b>                | <b>8</b> |

---

\*Electronic address: martin.hanczyc@unitn.it

†Electronic address: raffaello.potestio@unitn.it

‡Electronic address: roberto.menichetti@unitn.it

## I. EXPERIMENTAL SNAPSHOTS

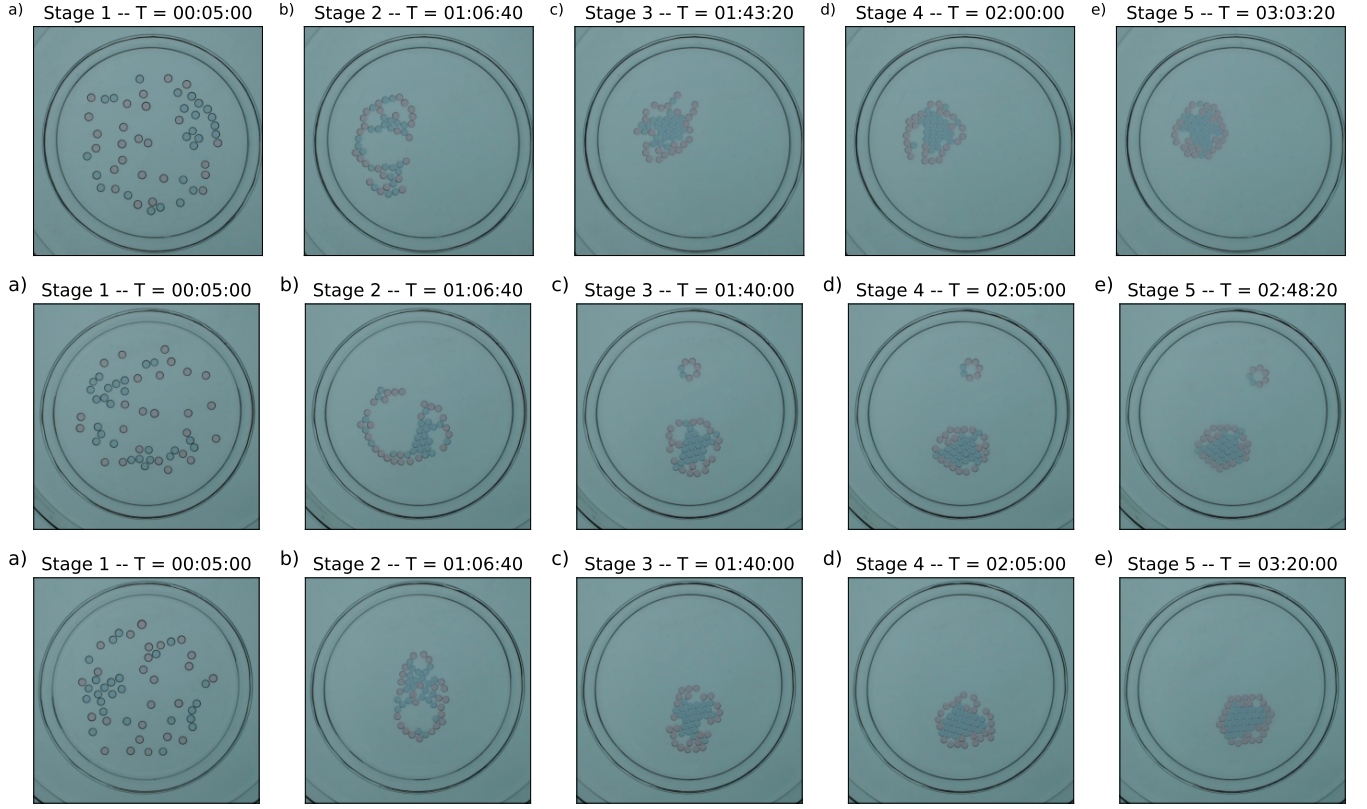

FIG. S1: From top to bottom: snapshots of the three experimental realizations of the system analyzed in this work illustrating typical droplet configurations at the onset of each evolutionary stage. Within each row (corresponding to an experiment), from left to right: Stage 1, high activity, disordered regime; Stage 2, intermediate self-propulsions and generation of transient structures; Stage 3, blue droplets cluster formed, disordered red droplets moving around it; Stage 4, red droplets start to cage the blue cluster; Stage 5, final “death” phase.

## II. COLLECTIVE VARIABLES ANALYSIS

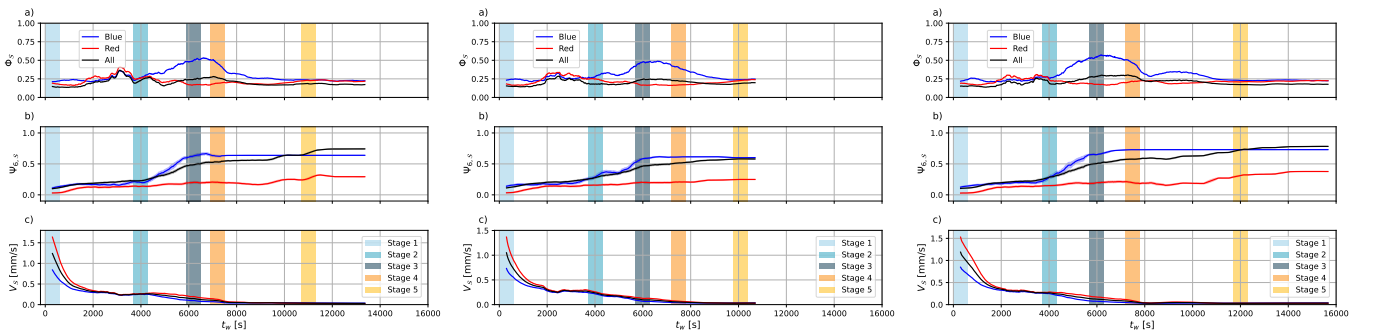

FIG. S2: From left to right: temporal evolution of the investigated collective variables for each of the three experimental realizations of the system analyzed in this work. Within each column (corresponding to an experiment), we report (a) the velocity polarization  $\Phi_S$ , (b) the hexatic order parameter  $\Psi_{6,S}$ , and (c) the average speed  $V_S$  of the blue droplet population (blue line), the red droplet population (red line), and overall droplet population (black line) as a function of the window running time  $t_w$ . In each experiment (columns), colored vertical bars indicate the onset of each evolutionary stage of the system.

### III. TIME- AND SPECIES-AVERAGED MEAN SQUARED DISPLACEMENTS

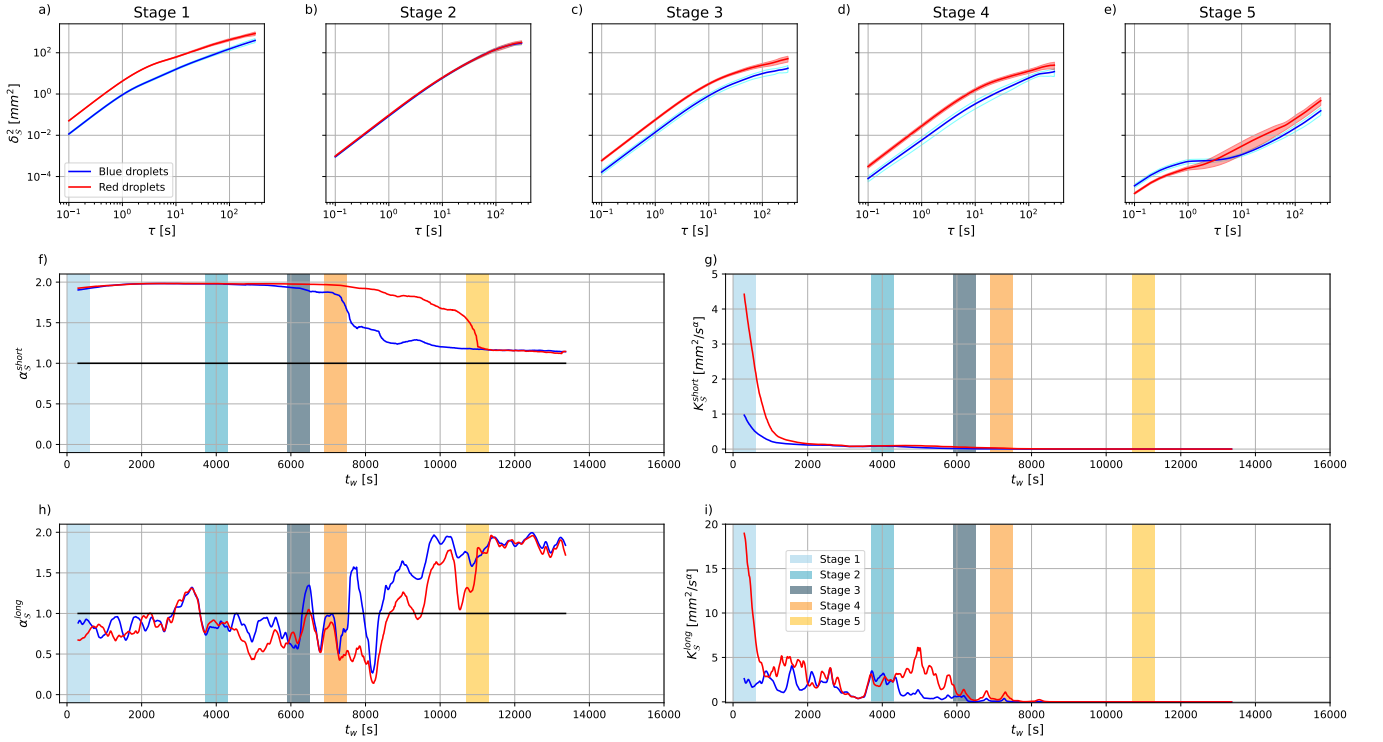

FIG. S3: Results for the time- and species-averaged mean squared displacements (TSAMSD) of the two droplet populations, see Eq. 9 of the main text, for the **first** experimental realization of the system analyzed in this work. (a-e) Progression from left to right illustrates the dependence of the family of  $\delta_S^2(\tau, t_w)$  TSAMSD curves on the lag time  $\tau$  for the blue (blue line) and red (red line) species at the onset of each evolutionary stage of the system—that is, for window times  $t_w$  located in the middle of each of the five colored vertical bars in the subsequent plots. (f-g) Temporal evolution of the short time-lag scaling exponents  $\alpha_S^{short}(t_w)$  and generalized diffusion coefficients  $K_S^{short}(t_w)$  of the two species, resulting from a power law fit, see Eq. 13 of the main text, of the family of  $\delta_S^2(\tau, t_w)$  profiles of the two species performed in the region  $\tau \in [0.1, 1]$  s. Colored vertical bars indicate the onset of each evolutionary stage. (h-i) Temporal evolution of the long-time lag scaling exponents  $\alpha_S^{long}(t_w)$  and generalized diffusion coefficients  $K_S^{long}(t_w)$  of the two species, obtained from a power law fit of the blue and red droplets TSAMSD performed in the region  $\tau \in [50, 300]$  s.

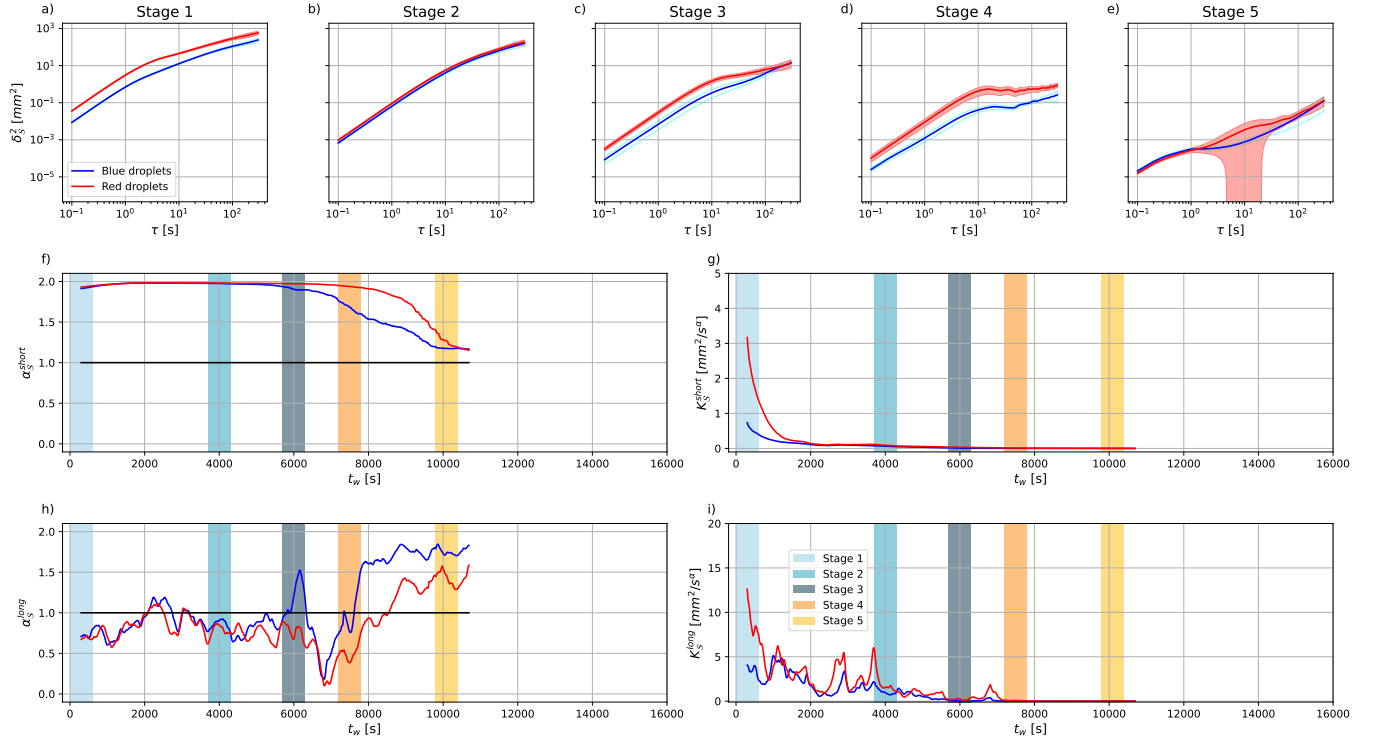

FIG. S4: Results for the time- and species-averaged mean squared displacements (TSAMSD) of the two droplet populations, see Eq. 9 of the main text, for the **second** experimental realization of the system analyzed in this work. (a-e) Progression from left to right illustrates the dependence of the family of  $\delta_S^2(\tau, t_w)$  TSAMSD curves on the lag time  $\tau$  for the blue (blue line) and red (red line) species at the onset of each evolutionary stage of the system—that is, for window times  $t_w$  located in the middle of each of the five colored vertical bars in the subsequent plots. (f-g) Temporal evolution of the short time-lag scaling exponents  $\alpha_S^{\text{short}}(t_w)$  and generalized diffusion coefficients  $K_S^{\text{short}}(t_w)$  of the two species, resulting from a power law fit, see Eq. 13 of the main text, of the family of  $\delta_S^2(\tau, t_w)$  profiles of the two species performed in the region  $\tau \in [0.1, 1]$  s. Colored vertical bars indicate the onset of each evolutionary stage. (h-i) Temporal evolution of the long-time lag scaling exponents  $\alpha_S^{\text{long}}(t_w)$  and generalized diffusion coefficients  $K_S^{\text{long}}(t_w)$  of the two species, obtained from a power law fit of the blue and red droplets TSAMSD performed in the region  $\tau \in [50, 300]$  s.

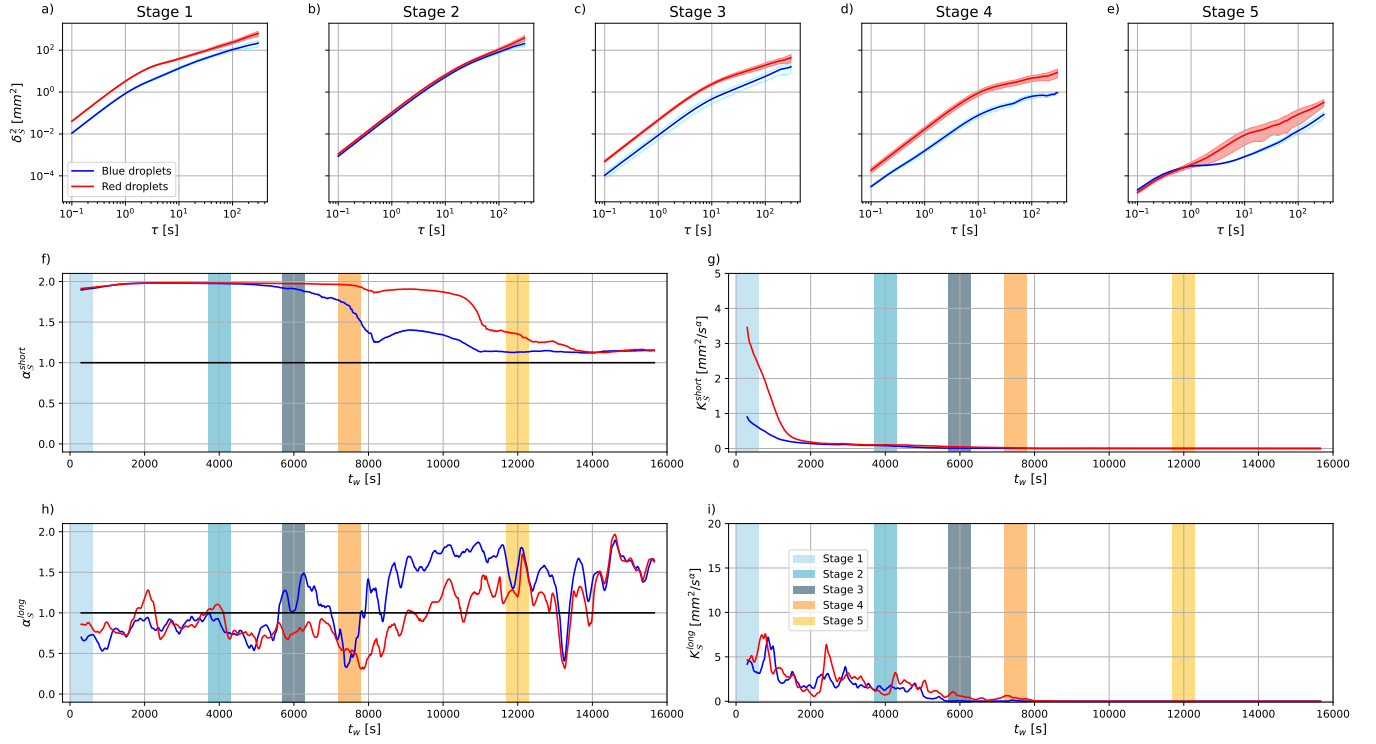

FIG. S5: Results for the time- and species-averaged mean squared displacements (TSAMSD) of the two droplet populations, see Eq. 9 of the main text, for the **third** experimental realization of the system analyzed in this work. (a-e) Progression from left to right illustrates the dependence of the family of  $\delta_S^2(\tau, t_w)$  TSAMSD curves on the lag time  $\tau$  for the blue (blue line) and red (red line) species at the onset of each evolutionary stage of the system—that is, for window times  $t_w$  located in the middle of each of the five colored vertical bars in the subsequent plots. (f-g) Temporal evolution of the short time-lag scaling exponents  $\alpha_S^{short}(t_w)$  and generalized diffusion coefficients  $K_S^{short}(t_w)$  of the two species, resulting from a power law fit, see Eq. 13 of the main text, of the family of  $\delta_S^2(\tau, t_w)$  profiles of the two species performed in the region  $\tau \in [0.1, 1]$  s. Colored vertical bars indicate the onset of each evolutionary stage. (h-i) Temporal evolution of the long-time lag scaling exponents  $\alpha_S^{long}(t_w)$  and generalized diffusion coefficients  $K_S^{long}(t_w)$  of the two species, obtained from a power law fit of the blue and red droplets TSAMSD performed in the region  $\tau \in [50, 300]$  s.

#### IV. VELOCITY AUTOCORRELATION FUNCTIONS

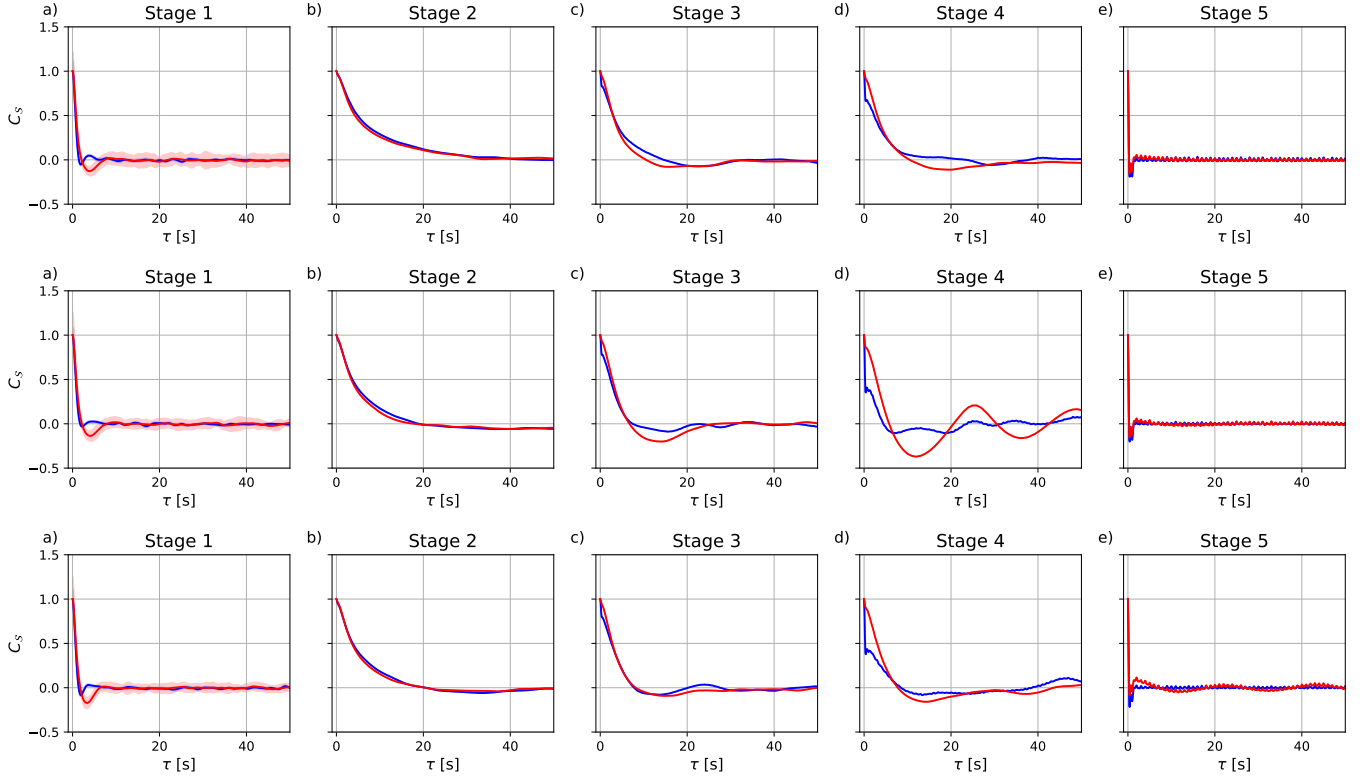

FIG. S6: From top to bottom: Velocity autocorrelation functions, see Eq. 10 of the main text, of the two droplet species for each of the three experimental realizations of the system analyzed in this work. Within each row (corresponding to one experiment): (a-e) Progression from left to right illustrates the  $\tau$ -dependence of the family of  $C_S(t_w, \tau)$  VACF curves for the blue (blue line) and red (red line) species at the onset of each evolutionary stage of the system—that is, for window times  $t_w$  located, in each experiment, in the middle of the corresponding set of five colored vertical bars in Fig. S2.

## V. TURNING ANGLE DISTRIBUTIONS

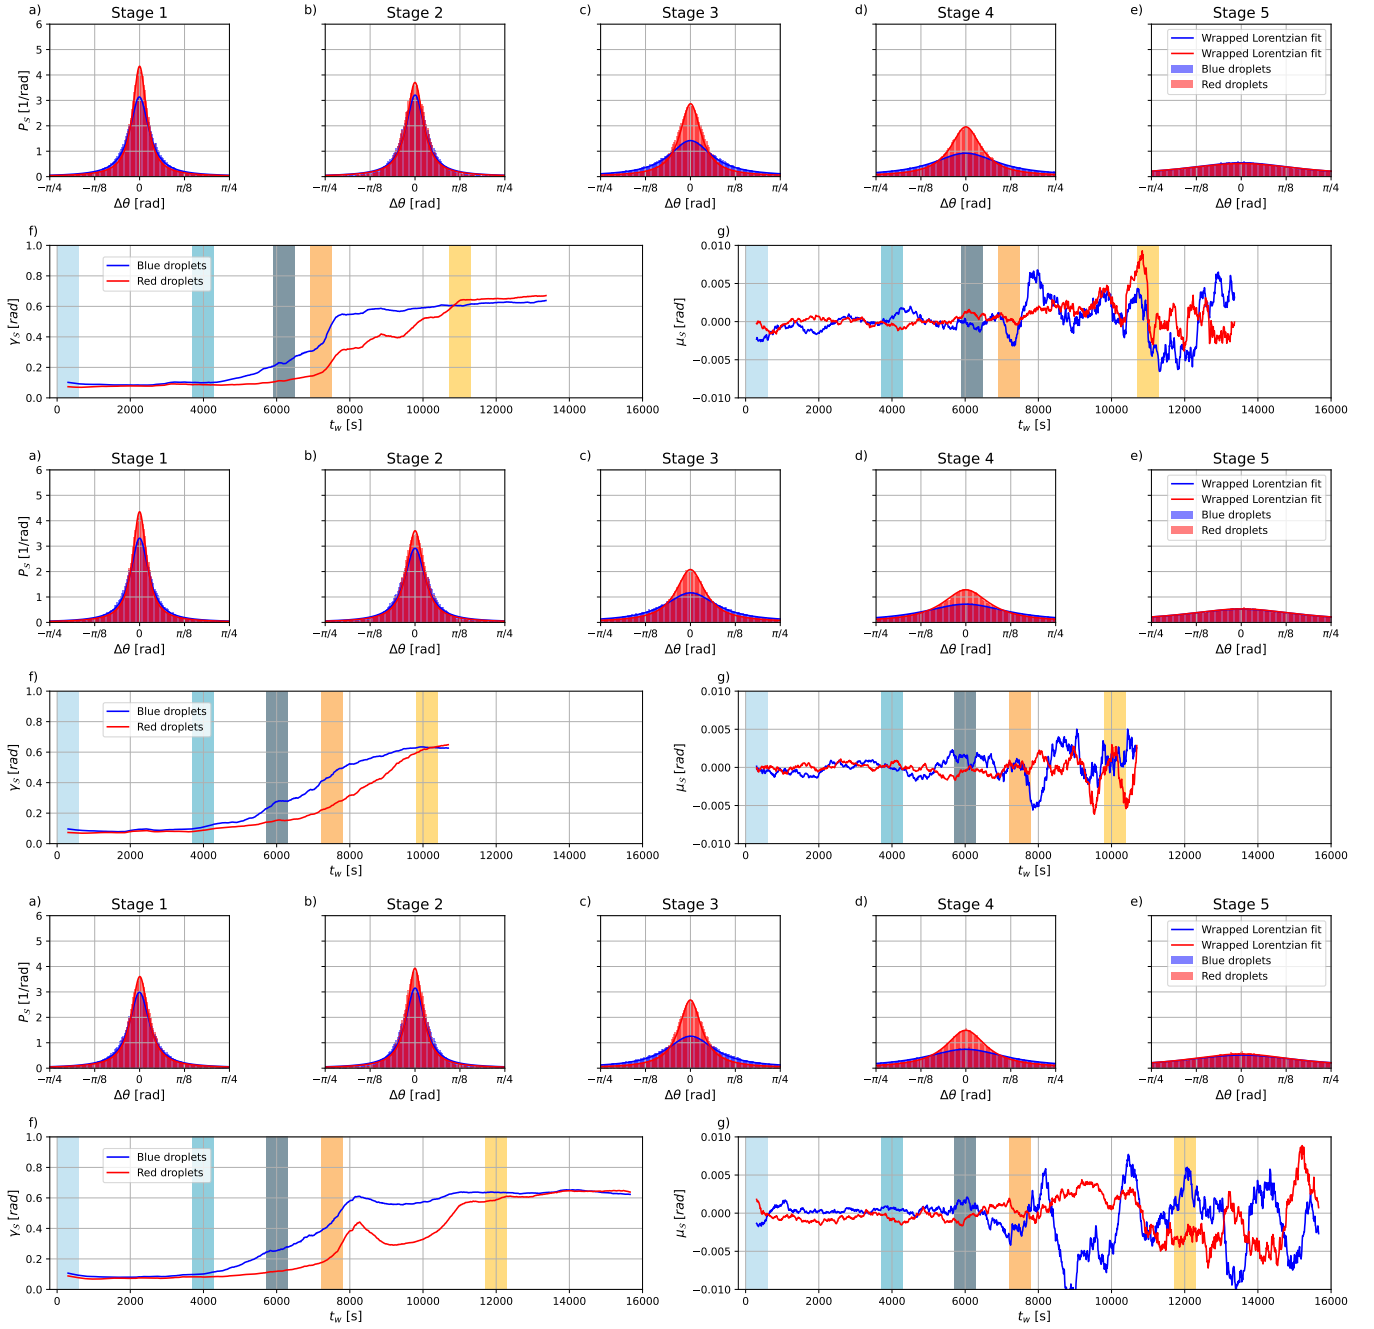

FIG. S7: From top to bottom: Turning angle distributions of the two droplet species, see Eq. 11 of the main text, for each of the three experimental realizations of the system analyzed in this work. In the panel of each experiment: (a-e) Progression from left to right illustrates the  $\Delta\theta$ -dependence of the family of  $P_S(\Delta\theta, t_w)$  turning angle distributions for the blue (blue line) and red (red line) species at the onset of each evolutionary stage of the system—that is, for window times  $t_w$  located in the middle of each of the five colored vertical bars in the subsequent plots. (f-g) Temporal evolution of the scale factor  $\gamma_S(t_w)$  and of the mean  $\mu_S(t_w)$  of the blue and red droplet species resulting from the wrapped Lorentzian fit of the family of  $P_S(\Delta\theta, t_w)$  profiles, see Eq. 14 of the main text. Colored vertical bars indicate the onset of each evolutionary stage.

## VI. DISTRIBUTION OF DROPLETS AROUND A DIMER

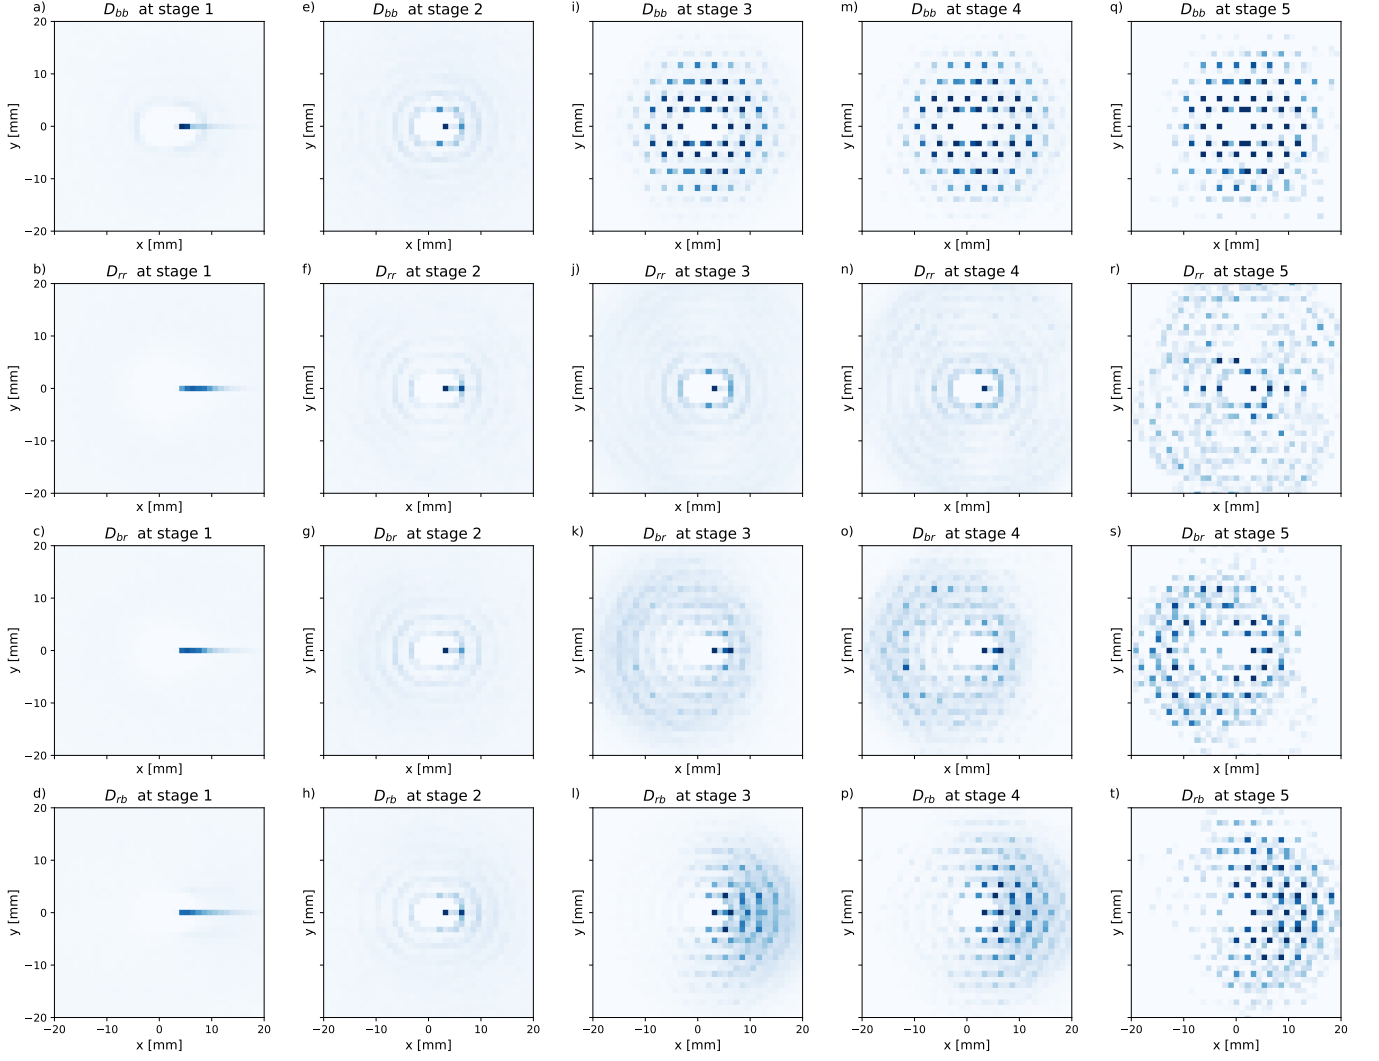

FIG. S8: The dimer distributions of the two droplet species defined in Eq. 12 of the main text, for the **first** experimental realization of the system analyzed in this work. In each column, from top to bottom: distributions between blue droplets  $D_{BB}$ , red droplets  $D_{RR}$ , blue-red droplets  $D_{BR}$ , red-blue droplets  $D_{RB}$ . In each row, from left to right: illustrative heat maps of the dimer distributions at the onset of each evolutionary stage of the system. Darker color indicates higher density (arbitrary units).



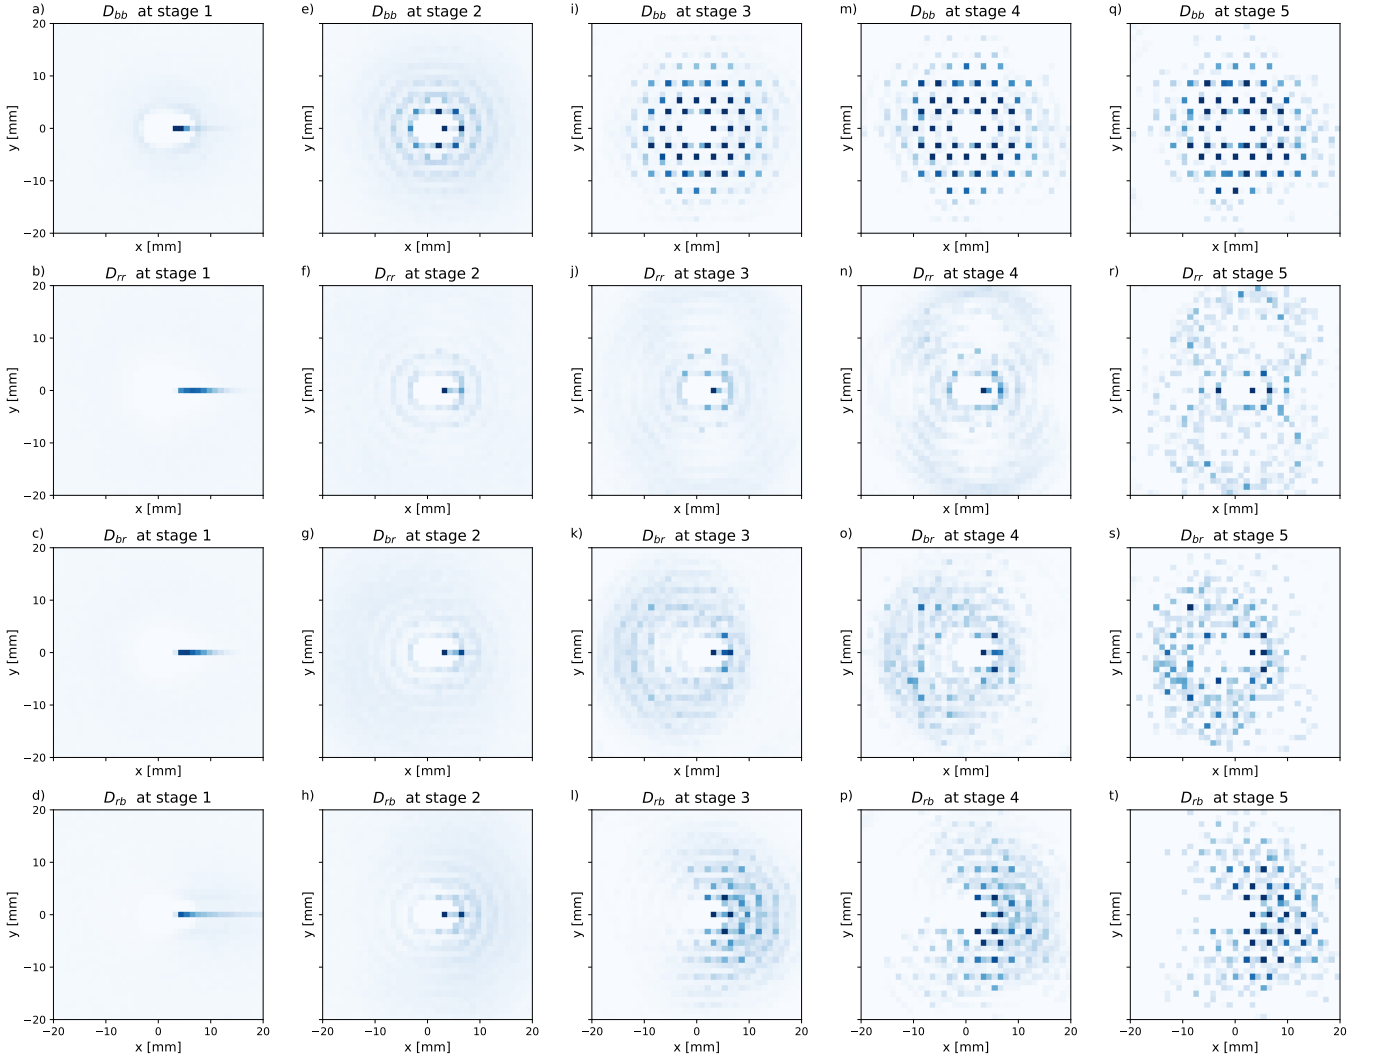

FIG. S9: The dimer distributions of the two droplet species defined in Eq. 12 of the main text, for the **second** experimental realization of the system analyzed in this work. In each column, from top to bottom: distributions between blue droplets  $D_{BB}$ , red droplets  $D_{RR}$ , blue-red droplets  $D_{BR}$ , red-blue droplets  $D_{RB}$ . In each row, from left to right: illustrative heat maps of the dimer distributions at the onset of each evolutionary stage of the system. Darker color indicates higher density (arbitrary units)

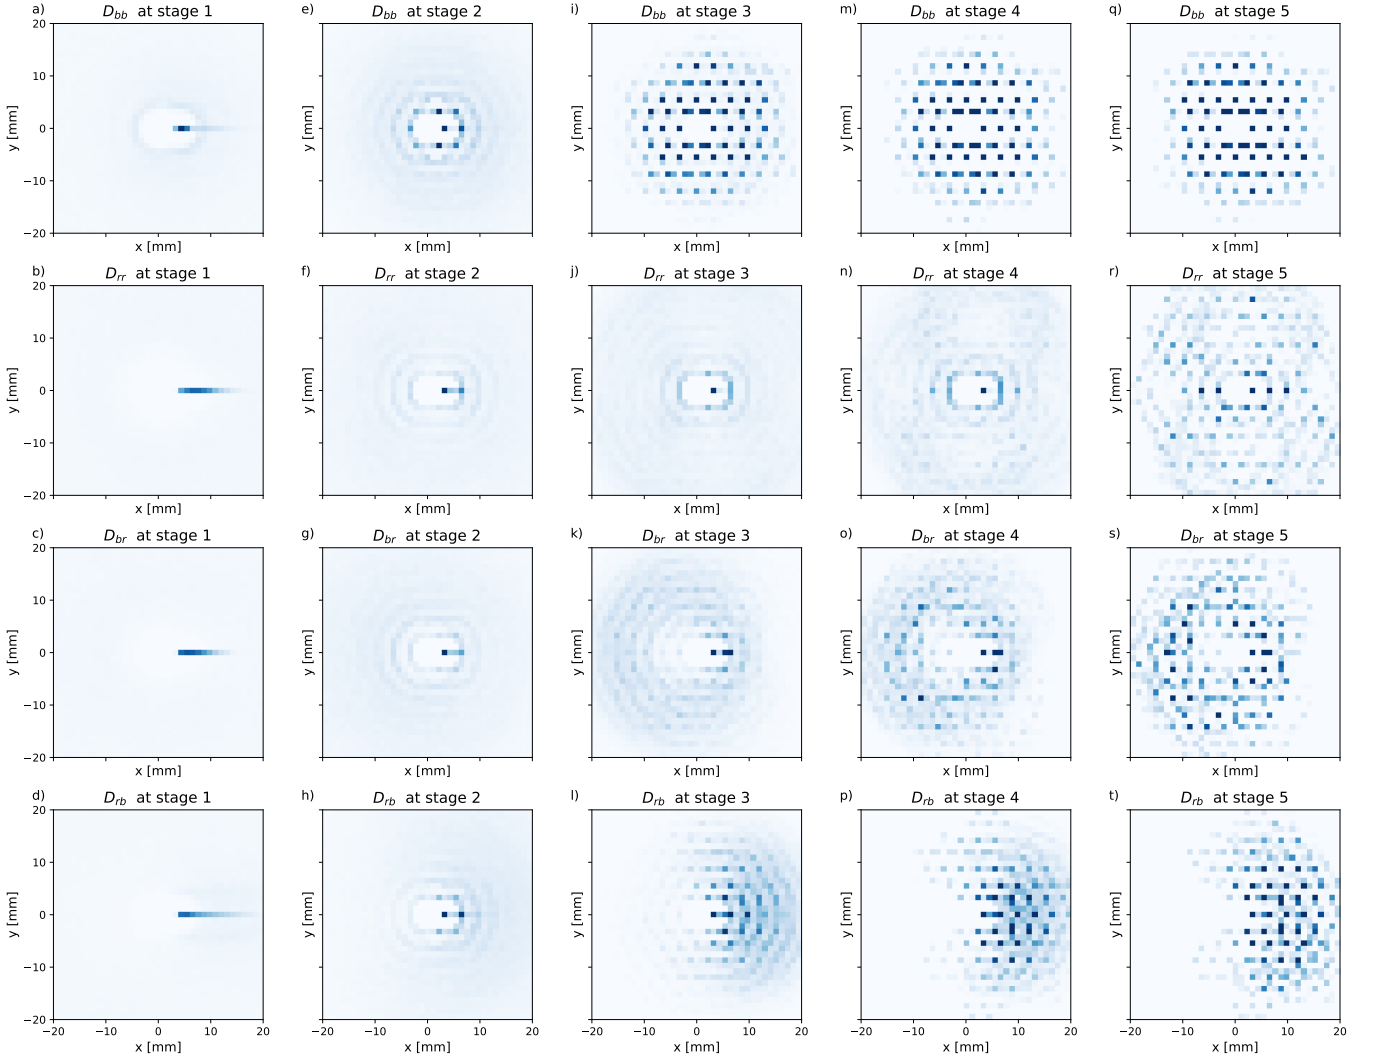

FIG. S10: The dimer distributions of the two droplet species defined in Eq. 12 of the main text, for the **third** experimental realization of the system analyzed in this work. In each column, from top to bottom: distributions between blue droplets  $D_{BB}$ , red droplets  $D_{RR}$ , blue-red droplets  $D_{BR}$ , red-blue droplets  $D_{RB}$ . In each row, from left to right: illustrative heat maps of the dimer distributions at the onset of each evolutionary stage of the system. Darker color indicates higher density (arbitrary units)
